# Supplementary material for: Eyemotion: Classifying facial expressions in VR using eye-tracking cameras
Source: arXiv:1707.07204 ancillary file (2017-07-28)
Supplement: Supplementary file 1 [file supp.pdf]

# **Eyemotion: Classifying facial expressions in VR using eye-tracking cameras**

## **Supplementary material**

### **1. Visual Examples**

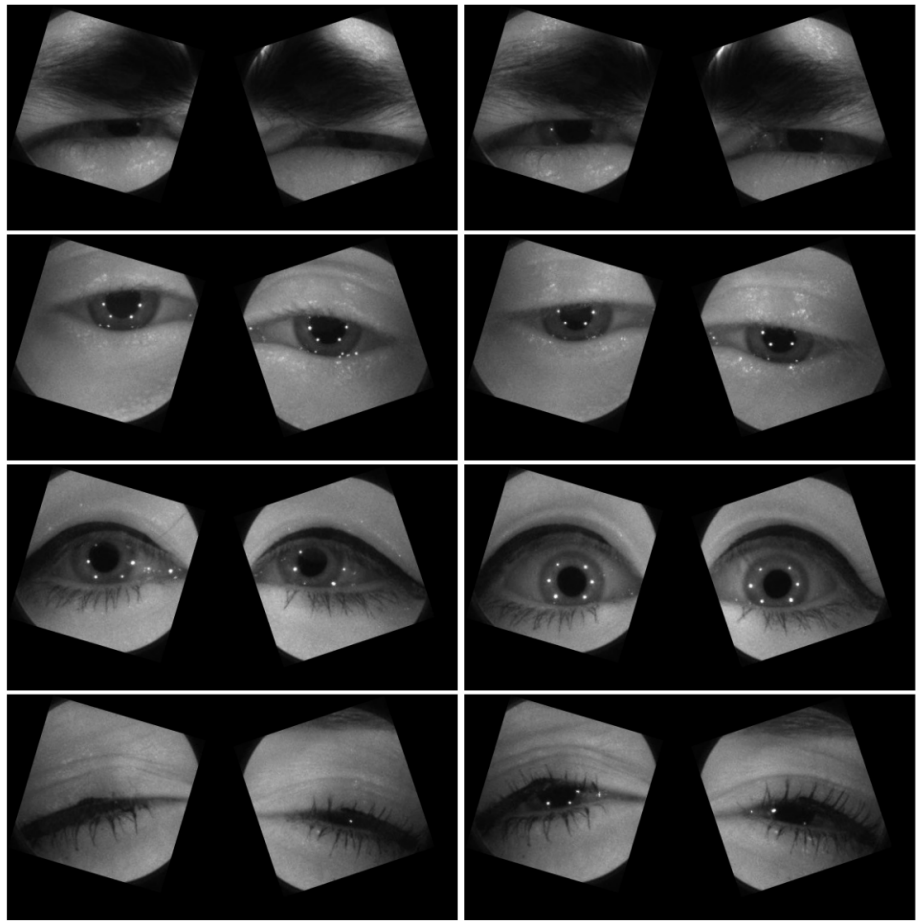

Figure 1: Example eye-images from four different users and expressions using HMD1. The expressions are (from top-to-bottom): anger, happiness, surprise, and squint. Similar images using HMD2 are shown in Fig. 2 of the paper. These images demonstrate the smaller field of view of eye images from HMD1.

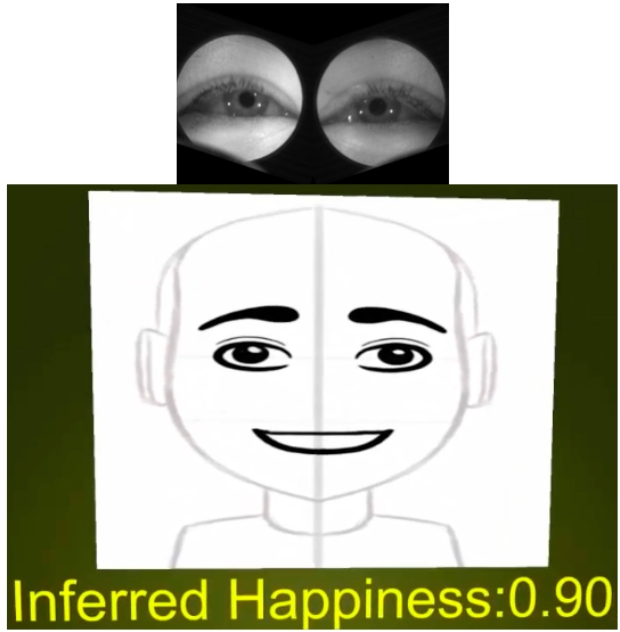

(a) Animation still with our model inferring happiness.

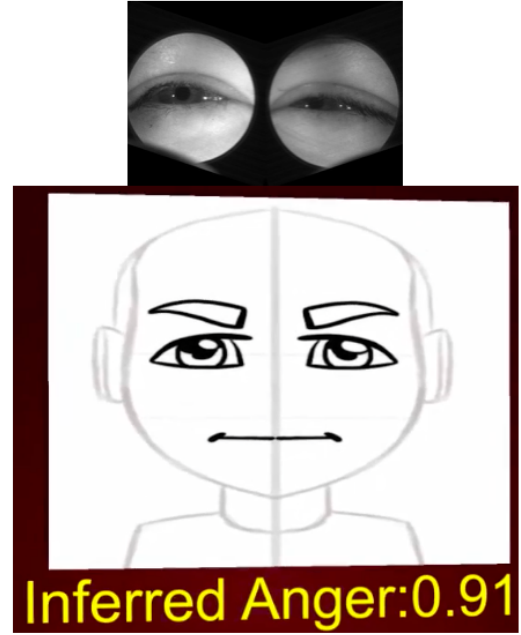

(b) Animation still with our model inferring anger.

Figure 2: Stills from an animation that can be driven by our model's inference as shown in our supplementary video. Top: Input eye images. Bottom: Inference demonstrated on a 2D avatar.

## 2. Classification Results

Next we show confusion matrices and classification reports for various experiments on classifying expressions from eye images from HMD1 and HMD2 using Eyemotion models. For the confusion matrices, labels are *Neutral (AU0)*, *Left Brow Raise (AU1+2L)*, *Right Brow Raise (AU1+2R)*, *Brow Lower (AU4)*, *Upper Lid Raise (AU5)*, *Squint (AU44)*, *Both Eyes Closed (AU43)*, *Left Wink (AU46L)*, *Right Wink (AU46R)*, and *Cheek Raise (AU6)*.

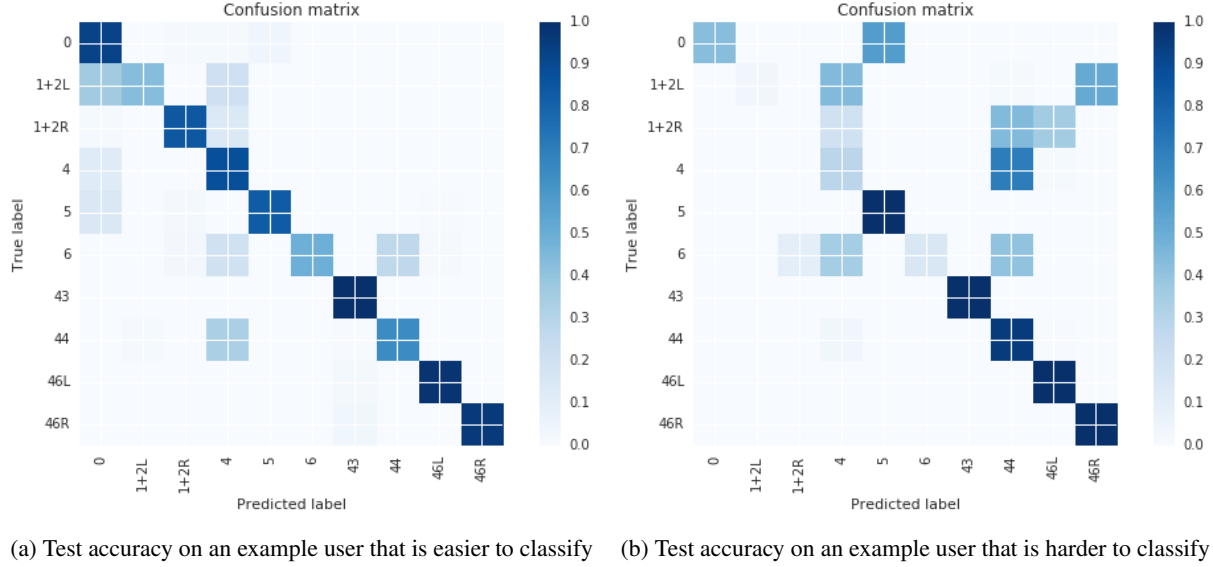

Figure 3: Confusion matrices for classification of facial action units using Inception V3 on HMD1 (without personalization) on (a) an easy to classify and (b) hard to classify single user.

| Expression       | Precision | Recall | $F_1$ | Support |
|------------------|-----------|--------|-------|---------|
| Brow lower       | 0.61      | 0.52   | 0.56  | 3129    |
| Brow raise       | 0.63      | 0.80   | 0.71  | 5438    |
| Cheek raise      | 0.31      | 0.37   | 0.33  | 2826    |
| Eyes closed      | 0.87      | 0.86   | 0.87  | 2882    |
| Left brow raise  | 0.58      | 0.36   | 0.45  | 2383    |
| Left wink        | 0.85      | 0.85   | 0.85  | 2451    |
| Neutral          | 0.52      | 0.45   | 0.49  | 3167    |
| Right brow raise | 0.49      | 0.38   | 0.43  | 1925    |
| Right wink       | 0.93      | 0.95   | 0.94  | 2600    |
| Squint           | 0.60      | 0.63   | 0.62  | 2701    |
| avg / total      | 0.64      | 0.64   | 0.63  | 29502   |

(a) Classification report. Overall mean accuracy 63.7%.

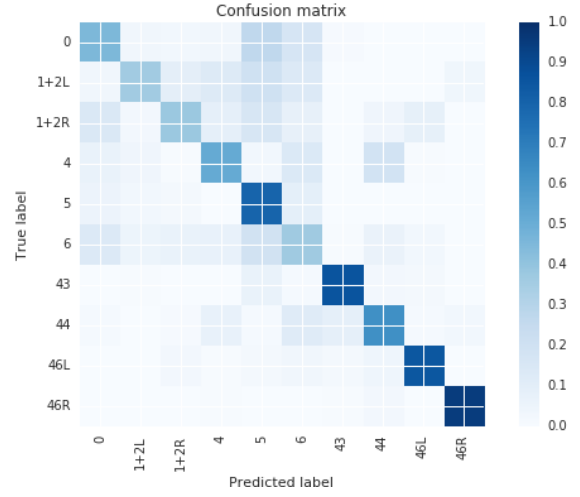

(b) Confusion matrix

Figure 4: Results for action unit classification, tested on held-out participants from HMD1, without using personalization.

| Expression       | Precision | Recall | $F_1$ | Support |
|------------------|-----------|--------|-------|---------|
| Brow lower       | 0.68      | 0.62   | 0.65  | 3031    |
| Brow raise       | 0.72      | 0.85   | 0.78  | 5250    |
| Cheek raise      | 0.70      | 0.40   | 0.50  | 2802    |
| Eyes closed      | 0.81      | 0.85   | 0.83  | 3038    |
| Left brow raise  | 0.54      | 0.36   | 0.43  | 2279    |
| Left wink        | 0.85      | 0.89   | 0.87  | 2568    |
| Neutral          | 0.61      | 0.92   | 0.74  | 3127    |
| Right brow raise | 0.49      | 0.41   | 0.45  | 2027    |
| Right wink       | 0.87      | 0.88   | 0.87  | 2732    |
| Squint           | 0.67      | 0.61   | 0.64  | 2648    |
| avg / total      | 0.70      | 0.71   | 0.70  | 29502   |

(a) Classification report. Overall mean accuracy 70.8%.

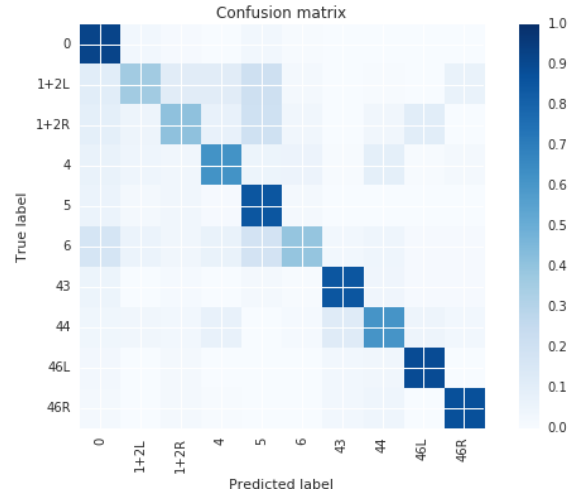

(b) Confusion matrix

Figure 5: Results for action units classification, tested on held-out participants from HMD1, with average-of-neutral-images personalization.

| Expression  | Precision | Recall | $F_1$ | Support |
|-------------|-----------|--------|-------|---------|
| Anger       | 0.75      | 0.70   | 0.72  | 2727    |
| Eyes Closed | 0.96      | 0.85   | 0.90  | 3211    |
| Happiness   | 0.40      | 0.43   | 0.41  | 3179    |
| Neutral     | 0.50      | 0.52   | 0.51  | 3040    |
| Surprise    | 0.53      | 0.57   | 0.55  | 3296    |
| avg / total | 0.63      | 0.61   | 0.62  | 15453   |

(a) Classification report. Overall mean accuracy 61.1%.

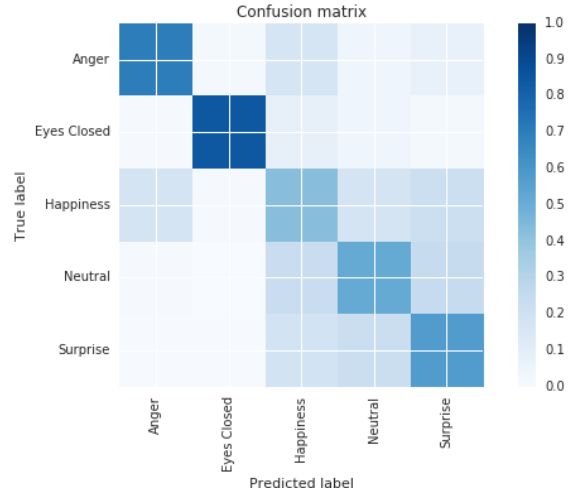

(b) Confusion matrix

Figure 6: Results for emotive expression classification, tested on held-out participants from HMD1, without using personalization.

| Expression  | Precision | Recall | $F_1$ | Support |
|-------------|-----------|--------|-------|---------|
| Anger       | 0.68      | 0.75   | 0.71  | 2826    |
| Eyes Closed | 0.87      | 0.76   | 0.81  | 2995    |
| Happiness   | 0.66      | 0.38   | 0.48  | 3172    |
| Neutral     | 0.67      | 0.94   | 0.78  | 3226    |
| Surprise    | 0.67      | 0.70   | 0.68  | 3234    |
| avg / total | 0.71      | 0.70   | 0.69  | 15453   |

(a) Classification report. Overall mean accuracy 70.3%.

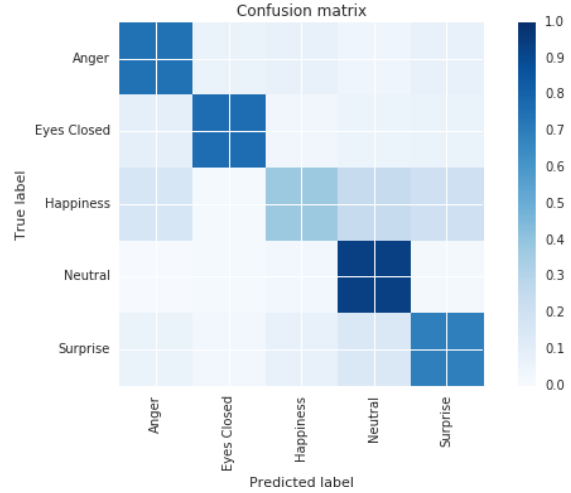

(b) Confusion matrix

Figure 7: Results for emotive expression classification, tested on held-out participants from HMD1, with average-of-neutral-images personalization.

| Action Unit      | Precision | Recall | $F_1$ | Support |
|------------------|-----------|--------|-------|---------|
| Brow lower       | 0.59      | 0.66   | 0.63  | 2897    |
| Upper lid raise  | 0.74      | 0.76   | 0.75  | 4912    |
| Cheek raise      | 0.56      | 0.64   | 0.60  | 2659    |
| Eyes closed      | 0.54      | 0.51   | 0.53  | 793     |
| Left brow raise  | 0.52      | 0.28   | 0.36  | 1598    |
| Left wink        | 0.95      | 0.86   | 0.90  | 2638    |
| Neutral          | 0.48      | 0.59   | 0.53  | 2309    |
| Right brow raise | 0.29      | 0.18   | 0.22  | 1855    |
| Right wink       | 0.83      | 0.87   | 0.85  | 2220    |
| Squint           | 0.62      | 0.71   | 0.66  | 2135    |
| Avg / total      | 0.64      | 0.65   | 0.64  | 24016   |

(a) Classification metrics. Overall mean accuracy 63.7%

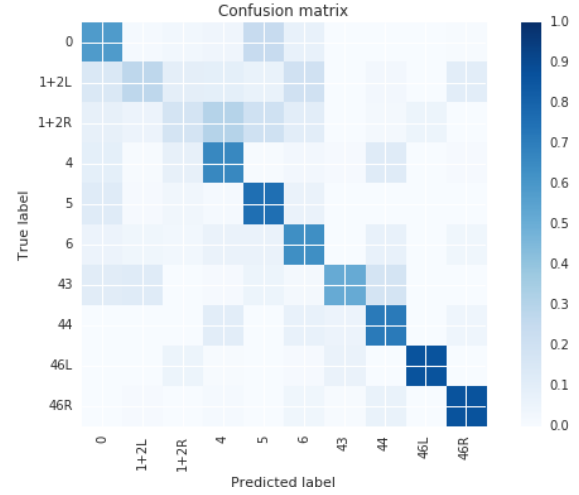

(b) Confusion matrix

Figure 8: Results for action unit classification, tested on held-out participants from HMD2, without using personalization.

| Action Unit      | Precision | Recall | $F_1$ | Support |
|------------------|-----------|--------|-------|---------|
| Brow lower       | 0.67      | 0.74   | 0.70  | 2576    |
| Upper lid raise  | 0.75      | 0.70   | 0.73  | 4956    |
| Cheek raise      | 0.65      | 0.64   | 0.64  | 2903    |
| Eyes closed      | 0.92      | 0.54   | 0.68  | 872     |
| Left brow raise  | 0.61      | 0.33   | 0.43  | 1616    |
| Left wink        | 0.93      | 0.90   | 0.91  | 2577    |
| Neutral          | 0.53      | 0.96   | 0.68  | 2372    |
| Right brow raise | 0.50      | 0.24   | 0.32  | 1701    |
| Right wink       | 0.82      | 0.87   | 0.84  | 2235    |
| Squint           | 0.65      | 0.67   | 0.66  | 2208    |
| Avg / total      | 0.70      | 0.69   | 0.68  | 24016   |

(a) Classification metrics. Overall mean accuracy 70.2%

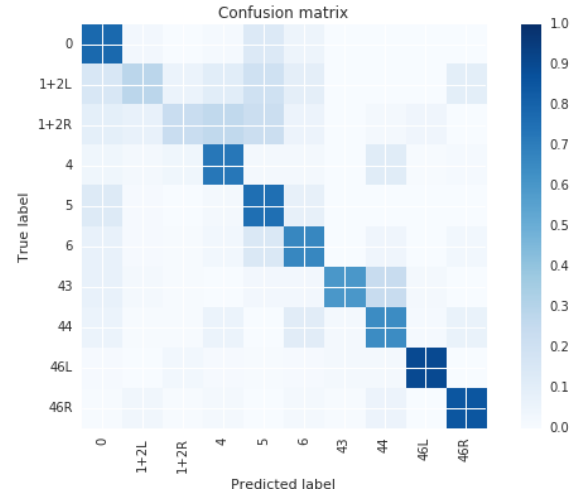

(b) Confusion matrix

Figure 9: Results for action unit classification, tested on held-out participants from HMD2, with average-of-neutral-images personalization.

| Expression  | Precision | Recall | $F_1$ | Support |
|-------------|-----------|--------|-------|---------|
| Anger       | 0.72      | 0.72   | 0.72  | 2695    |
| Closed Eyes | 0.77      | 0.78   | 0.77  | 899     |
| Happiness   | 0.66      | 0.67   | 0.66  | 2610    |
| Neutral     | 0.60      | 0.78   | 0.68  | 2274    |
| Surprise    | 0.71      | 0.51   | 0.59  | 2425    |
| avg / total | 0.68      | 0.68   | 0.67  | 10903   |

(a) Classification metrics. Overall mean accuracy 66.6%

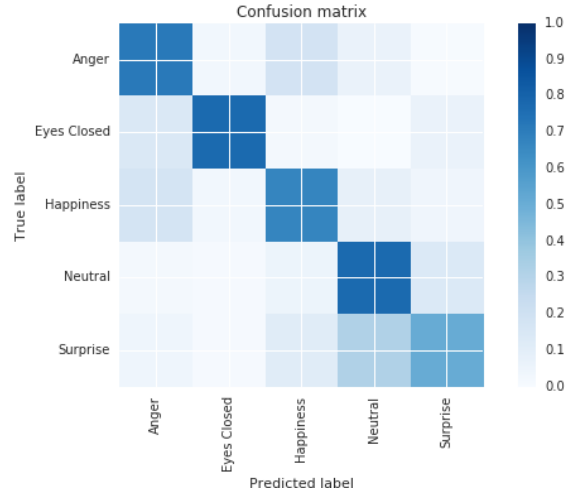

(b) Confusion matrix

Figure 10: Results for emotive expression classification, tested on held-out participants from HMD2, without using personalization.

| Expression  | Precision | Recall | $F_1$ | Support |
|-------------|-----------|--------|-------|---------|
| Anger       | 0.71      | 0.83   | 0.77  | 2455    |
| Closed Eyes | 0.90      | 0.67   | 0.77  | 863     |
| Happiness   | 0.81      | 0.60   | 0.69  | 2644    |
| Neutral     | 0.64      | 0.95   | 0.77  | 2425    |
| Surprise    | 0.81      | 0.60   | 0.69  | 2516    |
| avg / total | 0.76      | 0.74   | 0.73  | 10903   |

(a) Classification metrics. Overall mean accuracy 73.7%

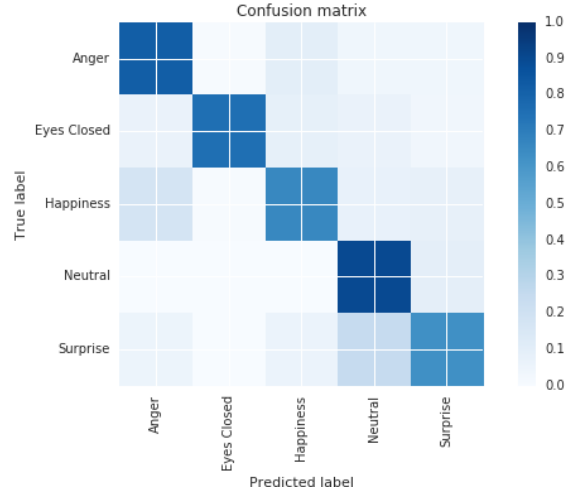

(b) Confusion matrix

Figure 11: Results for emotive expression classification, tested on held-out participants from HMD2, with average-of-neutral-images personalization.

| Expression       | Precision | Recall | $F_1$ | Support |
|------------------|-----------|--------|-------|---------|
| Brow lower       | 0.46      | 0.67   | 0.54  | 3422    |
| Brow raise       | 0.56      | 0.74   | 0.64  | 5974    |
| Cheek raise      | 0.44      | 0.50   | 0.47  | 3332    |
| Eyes closed      | 0.94      | 0.85   | 0.89  | 3450    |
| Left brow raise  | 0.79      | 0.35   | 0.48  | 5101    |
| Left wink        | 0.90      | 0.86   | 0.88  | 3081    |
| Neutral          | 0.35      | 0.40   | 0.38  | 3486    |
| Right brow raise | 0.71      | 0.48   | 0.57  | 4645    |
| Right wink       | 0.89      | 0.86   | 0.87  | 3121    |
| Squint           | 0.63      | 0.72   | 0.67  | 3124    |
| avg / total      | 0.66      | 0.63   | 0.63  | 38736   |

(a) Classification metrics. Overall mean accuracy 62.8%

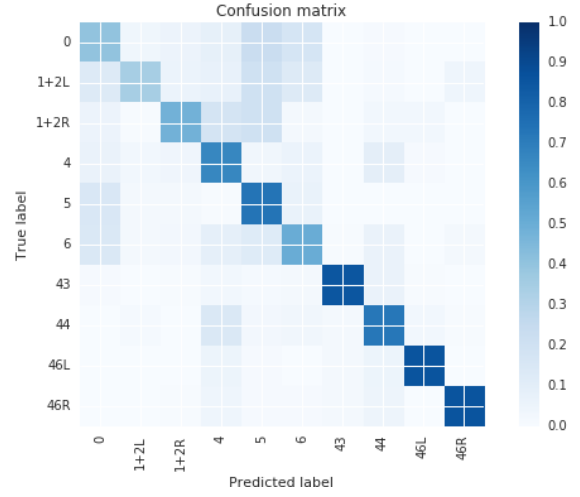

(b) Confusion matrix

Figure 12: Results for action unit classification, tested on held-out sessions from HMD1, without using personalization.

| Expression  | Precision | Recall | $F_1$ | Support |
|-------------|-----------|--------|-------|---------|
| Anger       | 0.83      | 0.77   | 0.80  | 3114    |
| Eyes Closed | 0.95      | 0.78   | 0.85  | 3689    |
| Happiness   | 0.63      | 0.68   | 0.65  | 3588    |
| Neutral     | 0.69      | 0.55   | 0.61  | 3478    |
| Surprise    | 0.50      | 0.68   | 0.58  | 3860    |
| avg / total | 0.71      | 0.69   | 0.69  | 17729   |

(a) Classification metrics. Overall mean accuracy 68.8%

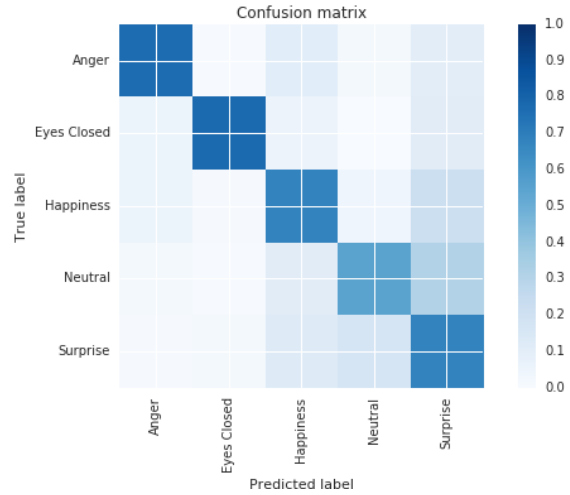

(b) Confusion matrix

Figure 13: Results for emotive expression classification, tested on held-out sessions from HMD1, without using personalization.

| Expression       | Precision | Recall | $F_1$ | Support |
|------------------|-----------|--------|-------|---------|
| Brow lower       | 0.68      | 0.96   | 0.80  | 3032    |
| Brow raise       | 0.77      | 0.89   | 0.83  | 5392    |
| Cheek raise      | 0.73      | 0.76   | 0.74  | 2926    |
| Eyes closed      | 0.98      | 0.86   | 0.92  | 974     |
| Left brow raise  | 0.75      | 0.59   | 0.66  | 2964    |
| Left wink        | 0.99      | 0.99   | 0.99  | 2725    |
| Neutral          | 0.69      | 0.70   | 0.70  | 2509    |
| Right brow raise | 0.90      | 0.53   | 0.67  | 3993    |
| Right wink       | 0.95      | 0.98   | 0.97  | 2562    |
| Squint           | 0.88      | 0.88   | 0.88  | 2628    |
| avg / total      | 0.82      | 0.81   | 0.80  | 29705   |

(a) Classification metrics. Overall mean accuracy 80.6%

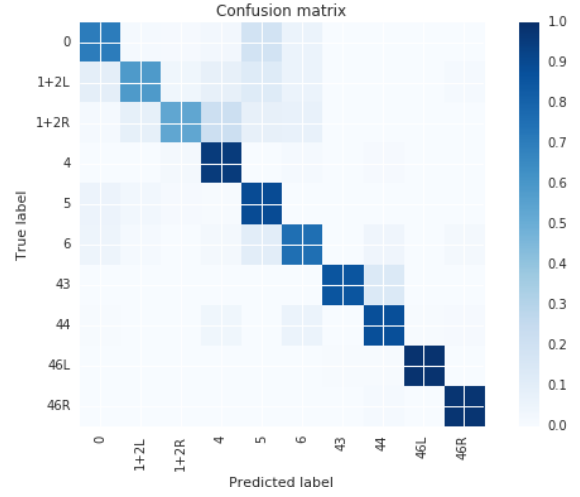

(b) Confusion matrix

Figure 14: Results for action unit classification, tested on held-out sessions from HMD2, without using personalization.

| Expression  | Precision | Recall | $F_1$ | Support |
|-------------|-----------|--------|-------|---------|
| Anger       | 0.91      | 0.93   | 0.92  | 2892    |
| Eyes Closed | 0.99      | 0.90   | 0.94  | 880     |
| Happiness   | 0.81      | 0.72   | 0.76  | 2969    |
| Neutral     | 0.77      | 0.92   | 0.84  | 2525    |
| Surprise    | 0.78      | 0.74   | 0.76  | 2642    |
| avg / total | 0.83      | 0.83   | 0.83  | 11908   |

(a) Classification metrics. Overall mean accuracy 83.2%

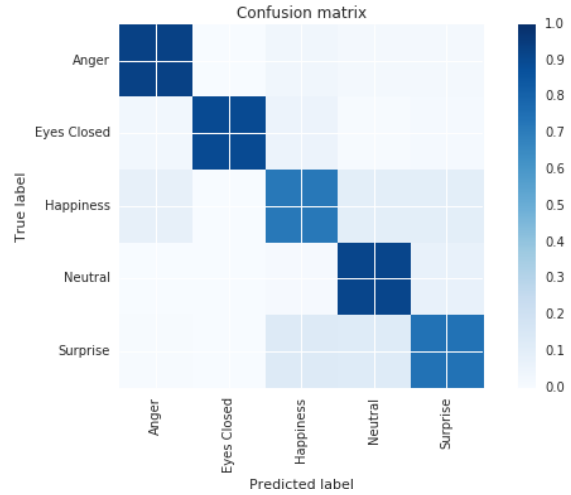

(b) Confusion matrix

Figure 15: Results for emotive expression classification, tested on held-out sessions from HMD2, without using personalization.
